# Supplementary material for: Parallel MMF: a Multiresolution Approach to Matrix Computation
Source: arXiv:1507.04396 source file (2015-07-15)
Supplement: Supplementary file 1 [file preconditioning.tex]

\documentclass[11pt,letterpaper]{article}
\usepackage[latin1]{inputenc}
\usepackage{amsmath}
\usepackage{amsfonts}
\usepackage{amssymb}
\usepackage{fullpage}
\usepackage{graphicx}
\begin{document}
	\section{Preconditioning experiments}
		We compared the performance of pMMF as a preconditioner for conjugate gradient method against the most commonly used preconditioners with standard settings. We compared with the Jacobi (diagonal) preconditioner, incomplete Cholesky decomposition and Symmetric successive over-relaxation (SSOR) with $\omega=1$. These methods are described in detail in 
		
		Jacobi preconditioner is a diagonal matrix whose entries are diagonals of $A$. In our code, we set the inverses of zero diagonal elements as zero. 
		
		Incomplete Cholesky decomposition produces a product $M=LL^T$ where $L$ is sparse. $M^{-1}x$ is then determined via back-substitution on the lower triangular matrix. In cases where the computation of the incomplete Cholesky factorization failed, we computed the factorization of a diagonally dominant version of the matrix. The exact command we used in MATLAB is: 

			\begin{verbatim}
				alpha=max(sum(abs(M),2)./diag(M));
				L=ichol(sparse(M),struct('type','ict','droptol',1e-3,'diagcomp',alpha));
			\end{verbatim}
			
		In computing the inverse of the core-diagonal matrix, we set all values on the diagonal less than $10^{-12}$ to zero. 

		Datasets were sourced from two different repositories. One set of matrices are from social network graphs from the SNAP database. The second set of matrices are from the Uflorida repo. Rectangular matrices were symmetrized by adding with the transpose. All the matrices are positive definite, albeit ill-conditioned.
		
		To generate each plot, we first computed the preconditioners and ran conjugate gradient method to solve $Ax=b$ for 20 randomly generated values of $b$. The residual values per iterate were then averaged over the 20 different runs. The vertical bars on the plots indicate standard deviation. Jacobi preconditioner performed bad on all the datasets, therefore for the sake of clarity in the plots, we excluded this preconditioner in the figures.
		
		\textbf{Comments: } No preconditioner stands out as the best. While SSOR performs well for a large number of datasets, it fails to even converge on datasets like Chebyshev2, Chebyshev3. It is interesting that, on these datasets, MMF is the only preconditioner which results in convergence. 
		
		MMF equals or outperforms incomplete Cholesky preconditioner in almost all the cases. Though computation of the latter is faster, in applications where this overhead cost is amortized, MMF would be a preferable choice. As is clear from the running times annotated in the plots, CG with MMF is always the fastest by a large margin. Thought it may take more number of iterations, in applications where running time is crucial, MMF is preferred.
		
		\begin{figure}[ht]
			\centering 
			\begin{minipage}[b]{0.5\linewidth}%[t]{0.3\textwidth}
				\includegraphics[width=\textwidth]{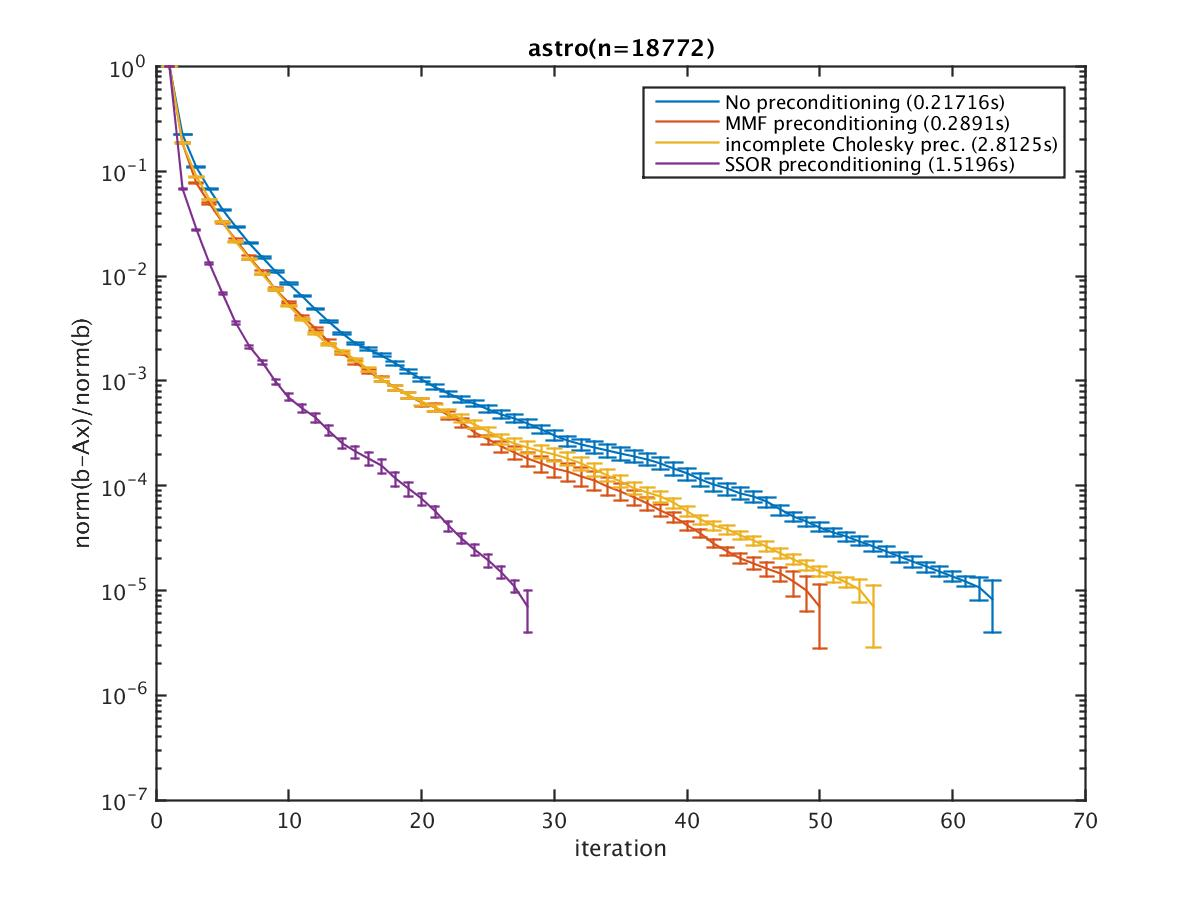}
				%\centering gnutella
				%\label{fig: HEP}
			\end{minipage}	
		\caption{\label{fig: linsolve} Performance of pMMF preconditioning in comparison to the ILU and SSOR preconditioners. }
		\end{figure}

	\begin{tabular}{r | l}
		Num. of stages & 15 \\
		Num. clusters & 2 \\
		Min. cluster size & 10 \\
		Max. cluster size & 5000/10000 \\
		Bypass cluster used? & yes \\
		Clustering recursion depth & 500 \\
		Givens rotations & yes \\
		Prenormalization & no \\
		Core matrix blocked? & no \\
		Normalize before selecting for rotations & yes \\
		Min. size of core & 10 \\
		Cols. eliminated per rotation & 1 \\
		Max. iterations of CG & 100 \\
		Tolerance & $10^{-5}$ \\
		Minimize off-diagonal norm? & yes 
	\end{tabular}

\end{document}
